# Supplementary material for: Data-Efficient Methods for Dialogue Systems
Source: arXiv:2012.02929 source file (2020-12-05)
Supplement: Supplementary file 1 [file AppendixX.tex]

% Appendix A

\chapter{Year 2018-19 results, plan for the next year} % Main appendix title

\label{AppendixX} % Change X to a consecutive letter; for referencing this appendix elsewhere, use \ref{AppendixX}

\lhead{Appendix X. \emph{Results, future work}} % Change X to a consecutive letter; this is for the header on each page - perhaps a shortened title

\section{Year 2018-19 results}

Over the third year of the PhD program, we have the following results:
\begin{itemize}
  \item The overall structure of the dissertation is outlined according to the main focus area, data-efficiency of dialogue systems (see the Table of Contents)
  \item A set of contributions have been made towards the dissertation goal. They are detailed below
  \item Several research papers have been submitted to the key conferences and workshops in dialogue systems area (see Appendix \ref{AppendixB}).
\end{itemize}

Having identified our main priority as improving robustness and data efficiency of dialogue systems \citep{Shalyminov.etal17}, in 2017 we made a contribution towards that goal: we presented a domain-general, generalisable and fully incremental disfluency detection model \citep{Shalyminov.etal18}.

In the year 2018-2019, we extended our research by focusing on two more key problems of practical data-efficiency. As part of a summer internship at Microsoft Research, we published two papers on the problem of detecting out-of-domain input and handling it in a robust way \citep{Shalyminov.etal18,LeeShalyminov2019}. After that, we proceeded to the most general and fundamental problem of data-efficiency: few-shot dialogue system bootstrapping. As such, we submitted papers for review to INTERSPEECH 2019, SigDial 2019, and EMNLP 2019 (see Appendix \ref{AppendixB}). Finally, we outlined our future work on integrating our individual contributions into the data-efficient dialogue systems suite as part of a research proposal for Facebook Robust Natural Language Processing grant (see Appendix \ref{AppendixB}). 

Apart from that, our research on data-efficient neural response ranking for socal conversation \citep{DBLP:conf/emnlp/ShalyminovDL18} was included in Alana team's Alexa Prize 2018 publication \citep{Curry.etal2018}.

\textbf{Improving Robustness of Neural Dialog Systems in a Data-Efficient Way with Turn Dropout}

Neural network-based dialog models often lack robustness to anomalous, out-of-domain (OOD) user input which leads to unexpected dialog behaviour and thus considerably limits such models' usage in mission-critical production environments. The problem is especially relevant in the setting of dialog system bootstrapping with limited training data and no access to OOD examples. In this paper, we explore the problem of robustness of such systems to anomalous input and the associated to it trade-off in accuracies on seen and unseen data. We present a new dataset for studying the robustness of dialog systems to OOD input, which is bAbI Dialog Task 6 augmented with OOD content in a controlled way.
We then present turn dropout, a simple  yet efficient negative sampling-based technique for improving robustness of neural dialog models. We demonstrate its effectiveness applied to Hybrid Code Network-family models (HCNs) which reach state-of-the-art results on our OOD-augmented dataset as well as the original one. Specifically, an HCN trained with turn dropout achieves state-of-the-art performance of more than \textbf{75\%} per-utterance accuracy on the augmented dataset's OOD turns and \textbf{74\%} F1-score as an OOD detector. Furthermore, we introduce a Variational HCN enhanced with turn dropout which achieves more than \textbf{56.5\%} accuracy on the original bAbI Task 6 dataset, thus outperforming the initially reported HCN's result.

The paper was presented at NeurIPS 2018 Workshop on Conversational AI as a \href{https://drive.google.com/file/d/1c6Kd3aGwaEj4tgyElIe1dYgAwM-B9aRd/view?usp=sharing}{poster}.

\textbf{Contextual out-of-domain utterance handling using counterfeit data augmentation}

As was showed in the previous paper, data augmentation can help increase dialogue systems' robustness to OOD input in a very data-efficient way, i.e. no training data was required apart from the system's trainset. However, the data augmentation procedure iteself can be further simplified by not generating the OOD input sequences and reducing them to a single number instead. For that, we used a separate component~--- an autoencoder~--- which would learn the distribution of the model's native in-domain train data during the pre-training stage. Then, it's plugged into the Hybrid Code Network model thus resulting in the AE-HCN model which we introduced as the dialogue model with increased OOD robustness. With this model, the autoencoder's input reconstruction score is passed into the HCN's architecture as an additional dialogue-level feature. And since autoencoder's reconstruction loss scores are known to be low for in-domain data and distinctively high for OOD data, direct training  on OOD turns in the Turn Dropout-like way becomes possible via providing synthetic reconstruction scores. We explored 2 variations of this architecture: with recurrent and convolutional autoencoder respectively. We showed that our method outperforms state-of-the-art dialog models equipped with a conventional OOD detection mechanism by a large margin in the presence of OOD utterances.

This paper was presented at ICASSP 2019 as an oral presentation.

\textbf{Few-shot dialogue generation without annotated data: a transfer learning approach}

Learning with minimal data is one of the key challenges in the development of practical, production-ready goal-oriented dialogue systems. In a real-world enterprise setting where dialogue systems are developed rapidly and are expected to work robustly for an ever-growing variety of domains, products, and scenarios, efficient learning from a limited number of examples becomes indispensable..
In this paper, we introduce a technique to achieve state-of-the-art dialogue generation performance in a few-shot setup, without using any annotated data. We do this by leveraging background knowledge from larger, more highly represented dialogue sources. We evaluate our model on the Stanford Multi-Domain Dialogue Dataset, consisting of human-human goal-oriented dialogues in in-car navigation, appointment scheduling, and weather information domains.
We show that our few-shot approach achieves state-of-the art results on that dataset by consistently outperforming the previous best model in terms of BLEU and Entity F1 scores, while being more data-efficient than it by not requiring any data annotation.

Variants of this paper were submitted to INTERSPEECH 2019, SigDial 2019, and EMNLP 2019.

\textbf{Alana v2: Entertaining and Informative Open-domain Social Dialogue using Ontologies and Entity Linking}

Heriot-Watt University's Alana team took part in the 2018 Alexa Prize in which it took the 3rd place prize. The main advances over the 2017 Alana system were: (1) a deeper Natural Language Understanding (NLU) pipeline; (2) the use of topic ontologies and Named Entity Linking to enable the user to navigate and search through a web of related information; (3) system generated clarification questions to interactively disambiguate between Named Entities as part of NLU; (4) a new profanity & abuse detection model with rule-based mitigation strategies; and (5) response retrieval from Reddit.

The paper also included our experiment on data-efficient neural response ranking for social conversation \citep{DBLP:conf/emnlp/ShalyminovDL18} where we showed that it's possible to obtain competitive response ranking performance only using raw unannotated dialogue transcripts.

This paper was part of the 2018 Alexa Prize Proceedings.

\section{Plan for the year 2019-20}

In the final year of the PhD program, we plan to accomplish the following items:

\textbf{Data-efficient user simulation for goal-oriented dialogue}

\textit{This project is supposed to be part of an internship at Microsoft Research Montréal during the summer of 2019.}

We plan to extend the impact of our work on data-efficient dialogue system design by applying our readily available data and techniques to alternative dialogue system training methodologies. Specifically, we plan to make a contribution to Reinforcement Learning-based dialogue systems by developing a technique to train data-efficient user simulation models with the ability to rapidly adapt to new dialogue domains.

We ware going to use the Maluuba MetaLWOz dataset with its 51 domain as our target dataset, and publicly available domain-general data (e.g. Reddit conversations) as the source dataset, and will work on developing a generative user simulation model able to maintain fluent and coherent in-domain goal-oriented dialogue with minimal training data required.

\textbf{Improving few-shot dialogue generation}

Our transfer learning-based approach, although being technically state-of-the-art for the Stanford Multi-Domain dialogue dataset, isn't ready for immediate adoption in industry because of its moderate numbers, e.g. BLEU and Entity F1 scores.   
Therefore, one of our main priorities is to make our contribution in this direction more complete and increase the overall system's performance to increase its potential practical impact. We plan to do that by approaching the few-shot dialogue generation problem as a 2-stage process: (1) generation of a delexicalised response template and (2) filling in the entities from the Knowledge Base, again in an end-to-end generative way.

Our initial experiments show that generic delexicalised response generation (stage 1) can work quite efficiently in a few-shot setup.
For the stage 2, we are building Knowledge Base controller model based on the ideas of 2 highly successful models, both  widely adopted in NLP: Key-Value Memory Networks~--- for selecting the most relevant row from the KB snippet, and Pointer Networks~--- for picking fields from it into the final response.

\textbf{Finalising the thesis}

In the final version of the thesis, we will extend the literature review for more broad coverage of the dialogue system research and identifying the place for our work in it. Also we will integrate our individual contributions made over the course of the PhD program into a cohesive narrative~--- following the overall structure we outlined in the Table of Contents.
