# Supplementary material for: Data-Efficient Methods for Dialogue Systems
Source: arXiv:2012.02929 source file (2020-12-05)
Supplement: Supplementary file 2 [file AppendixY.tex]

% Appendix B

\chapter{Submitted papers} % Main appendix title

\label{AppendixY} % For referencing this appendix elsewhere, use \ref{AppendixA}

\lhead{Appendix Y. \emph{Submitted papers}} % This is for the header on each page - perhaps a shortened title

\includepdf[pages=-,offset=75 -75]{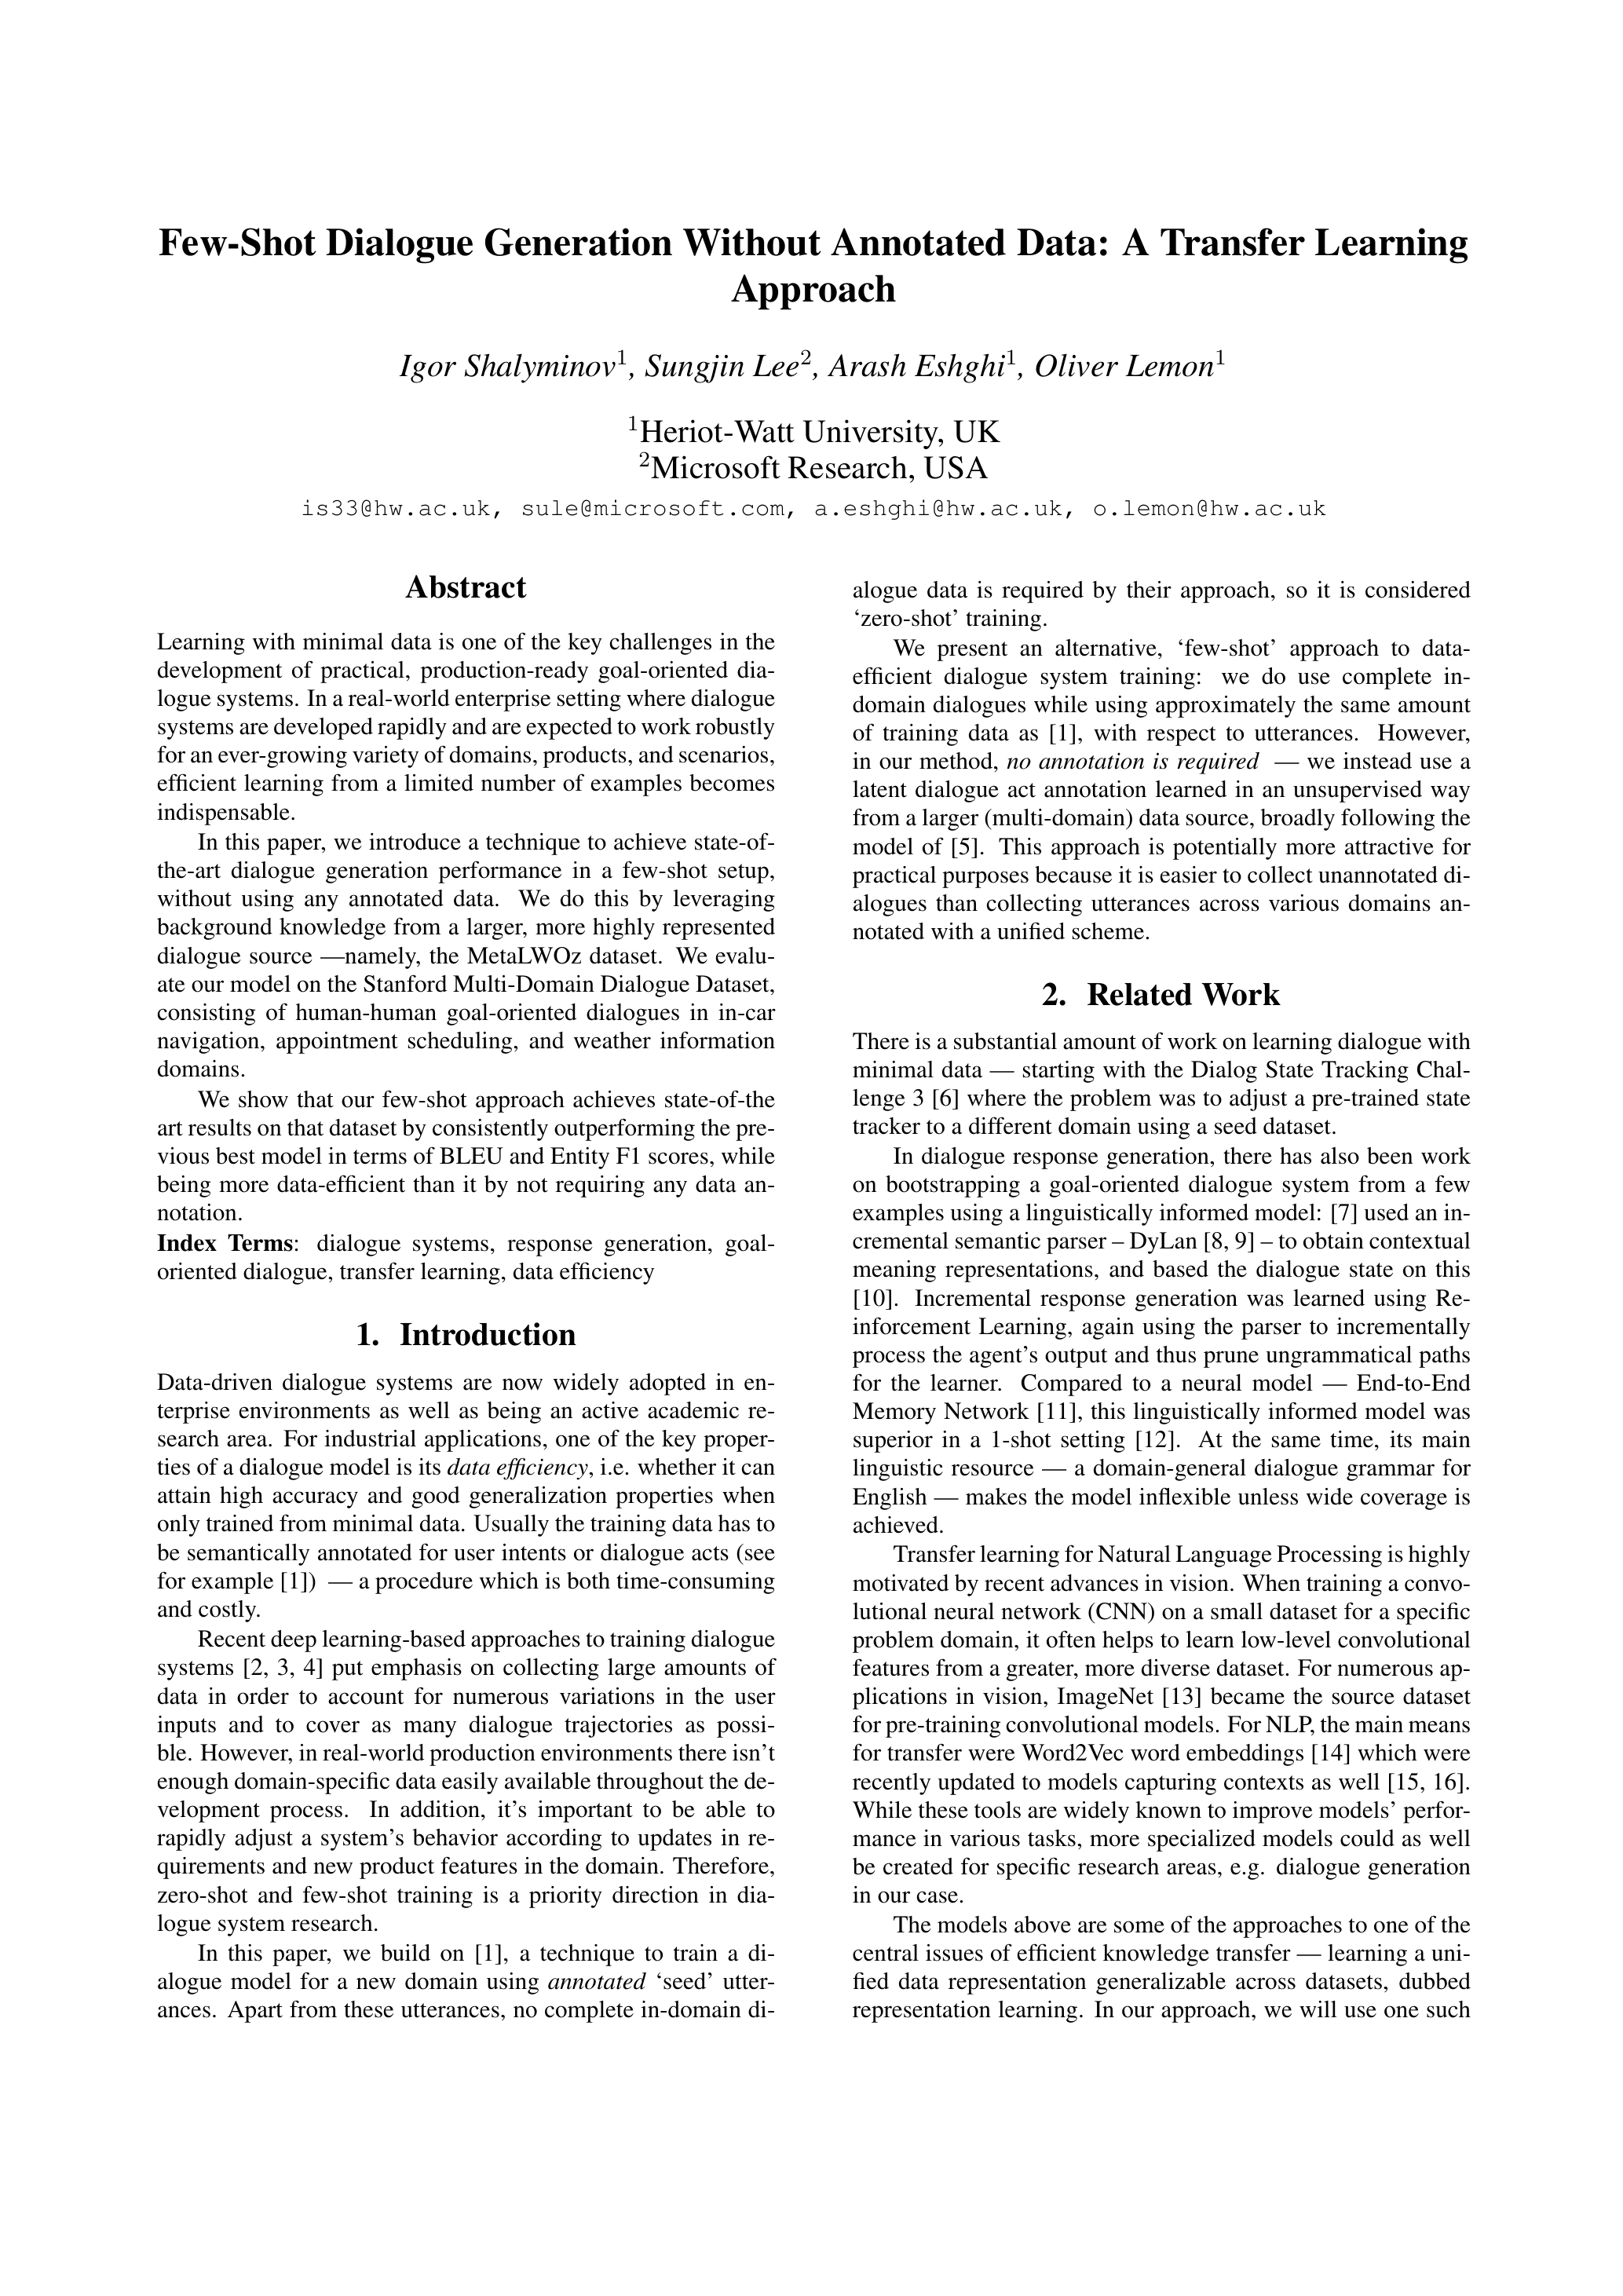}
% \includepdf[pages=-,offset=75 -75]{Papers/_SigDial_2019__Few_Shot_Dialogue_Generation_Without_Annotated_Data__A_Transfer_Learning_Approach.pdf}
\includepdf[pages=-,offset=75 -75]{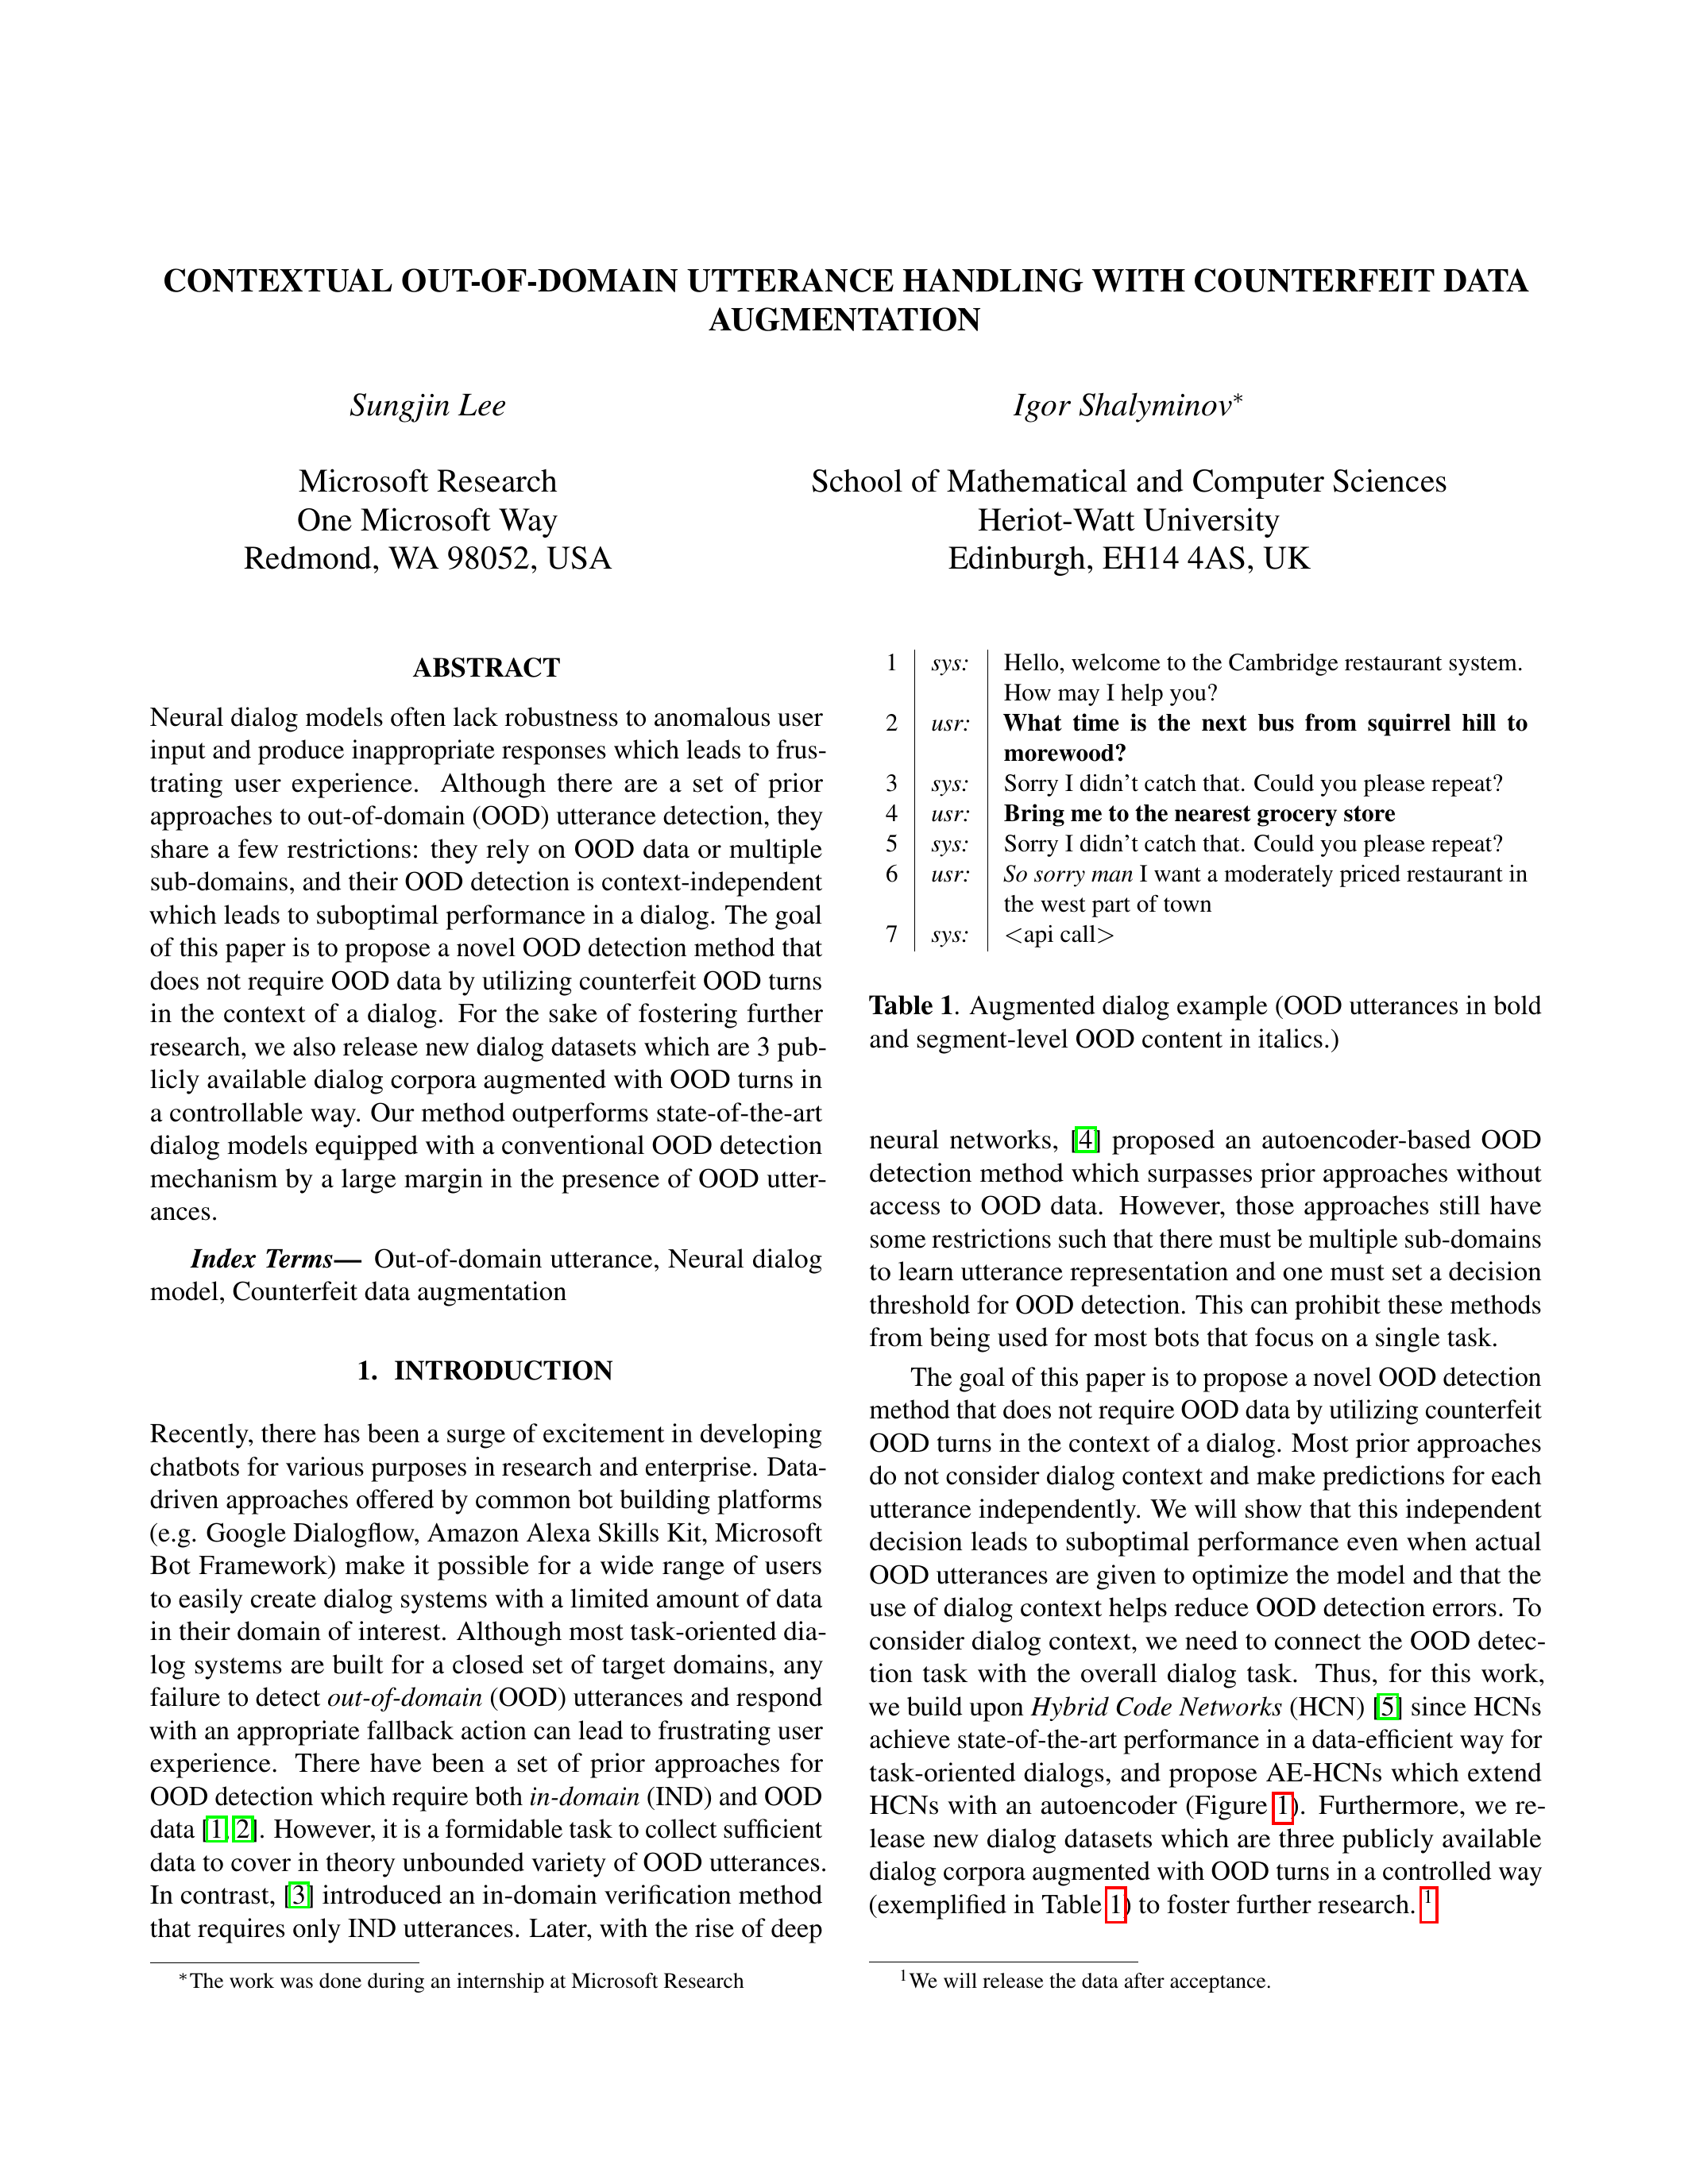}
\includepdf[pages=-,offset=75 -75]{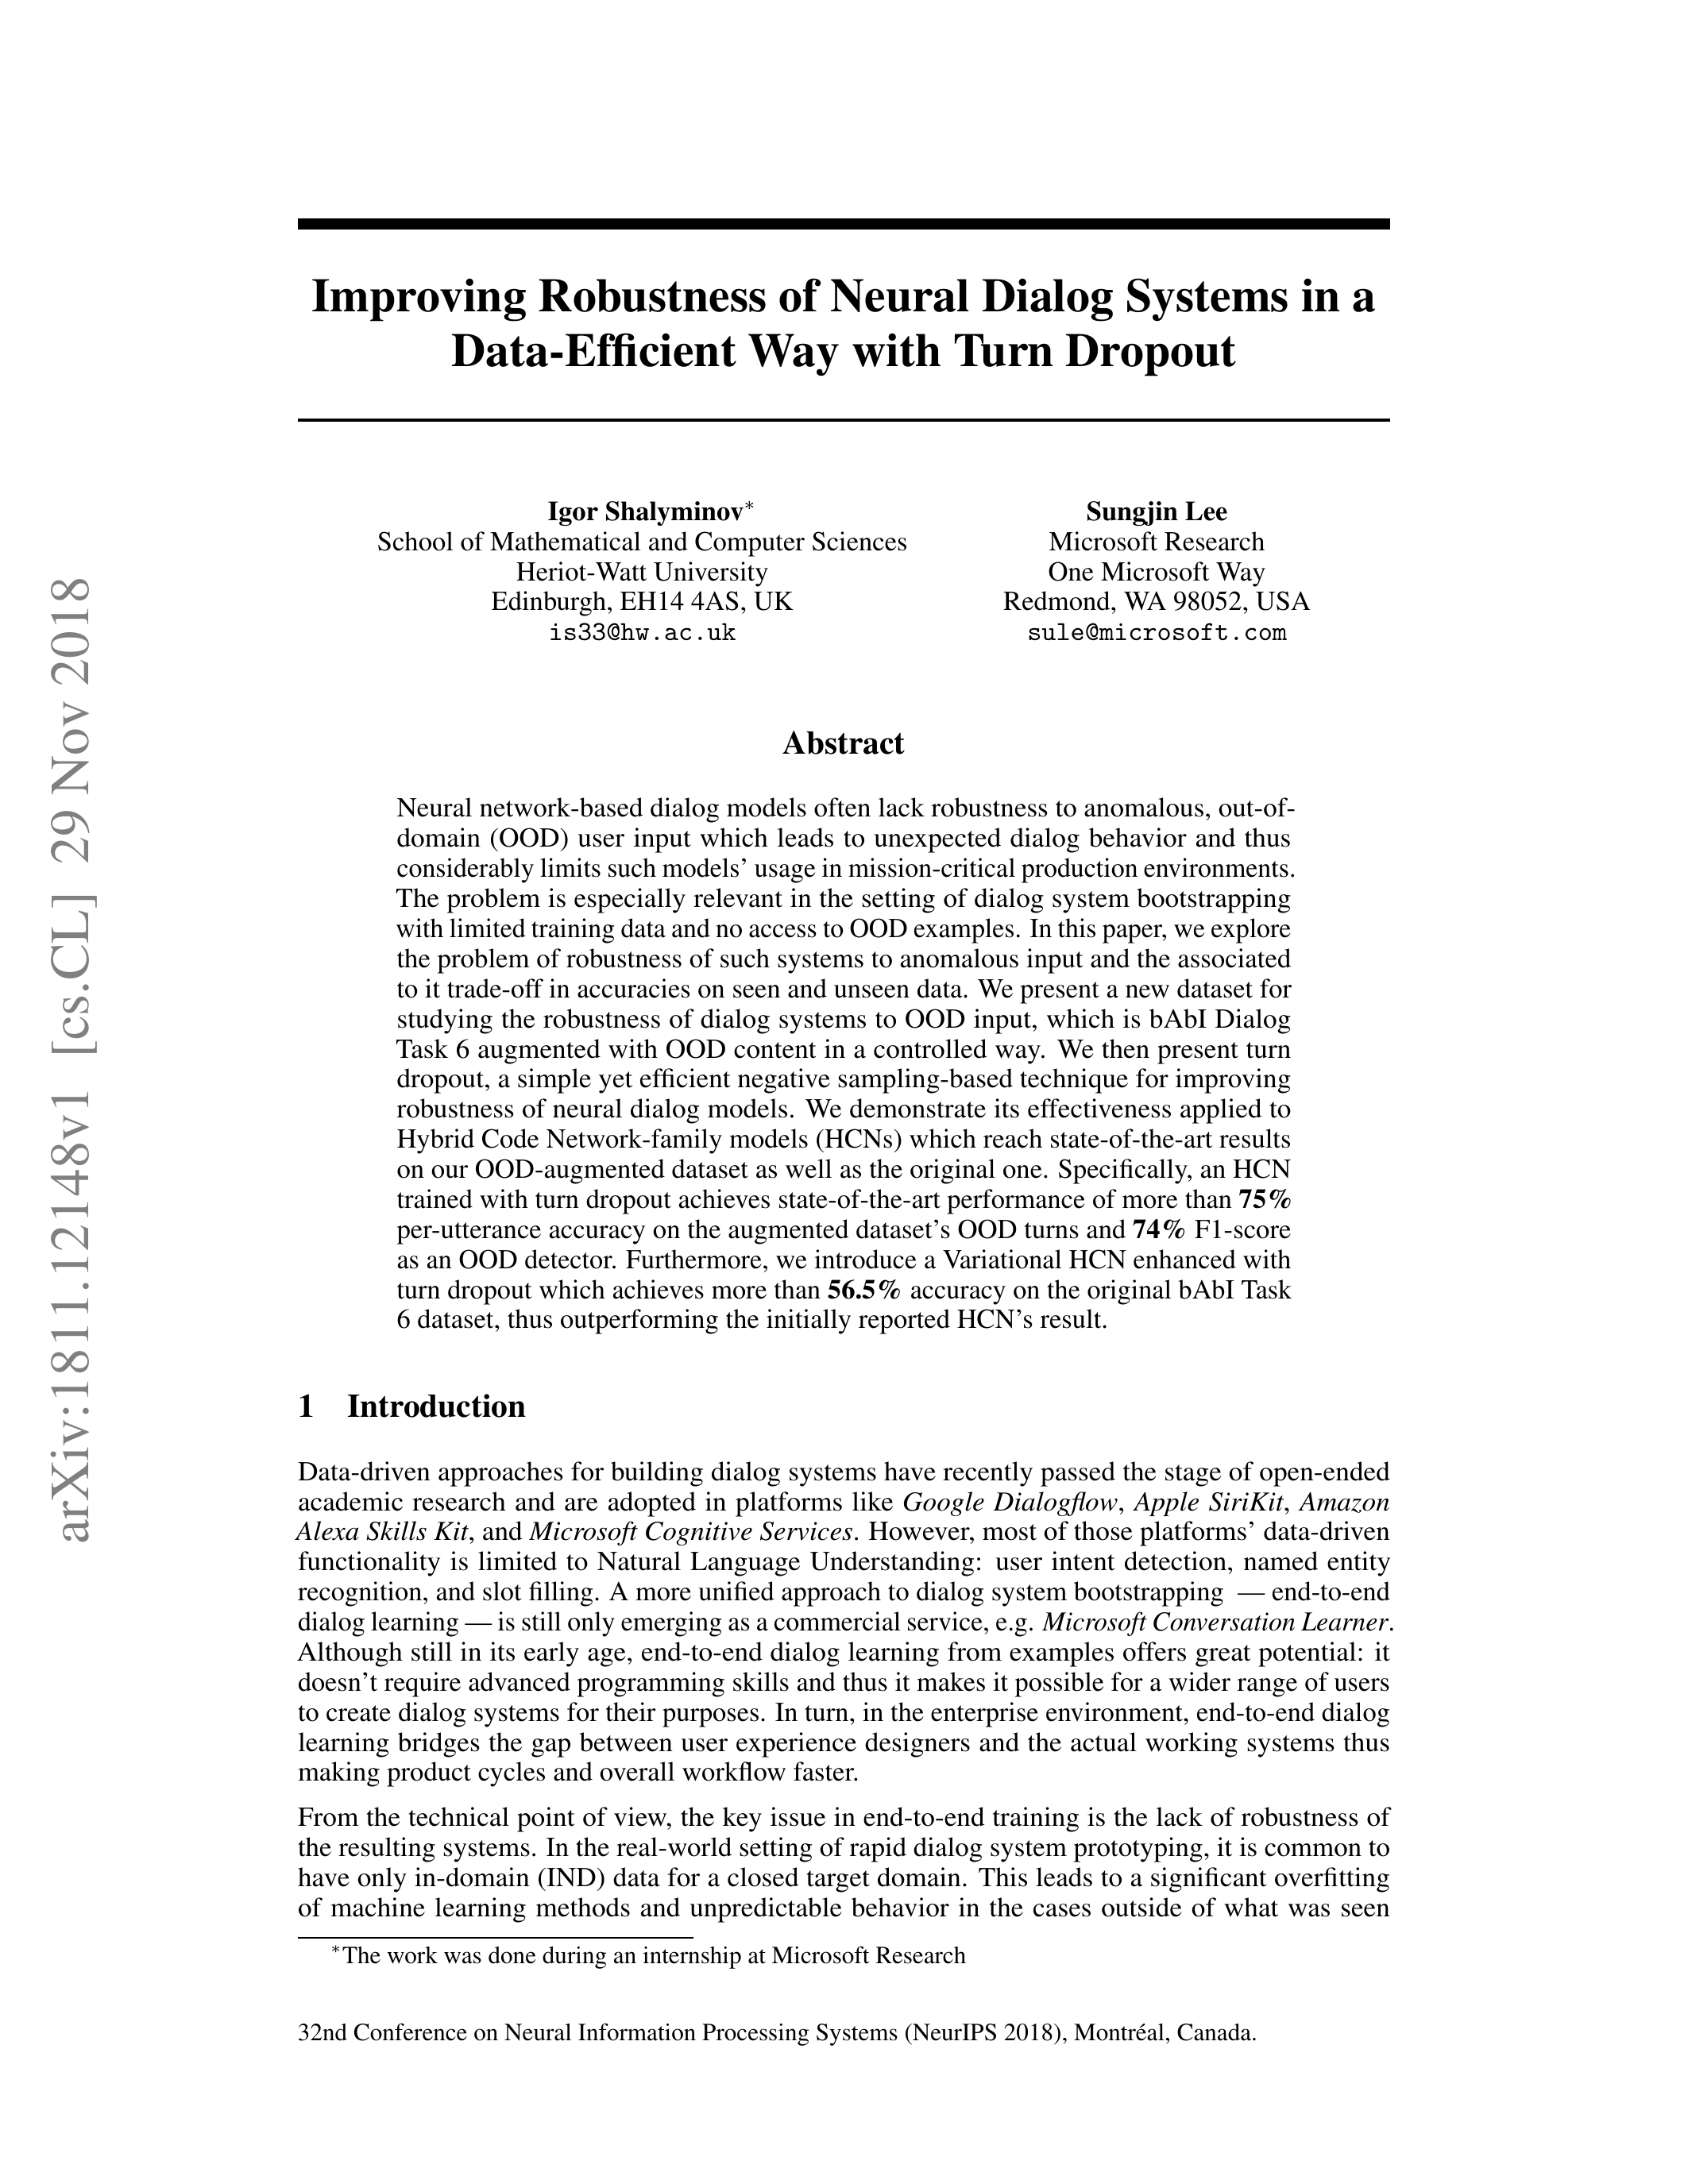}
\includepdf[pages=-,offset=75 -75]{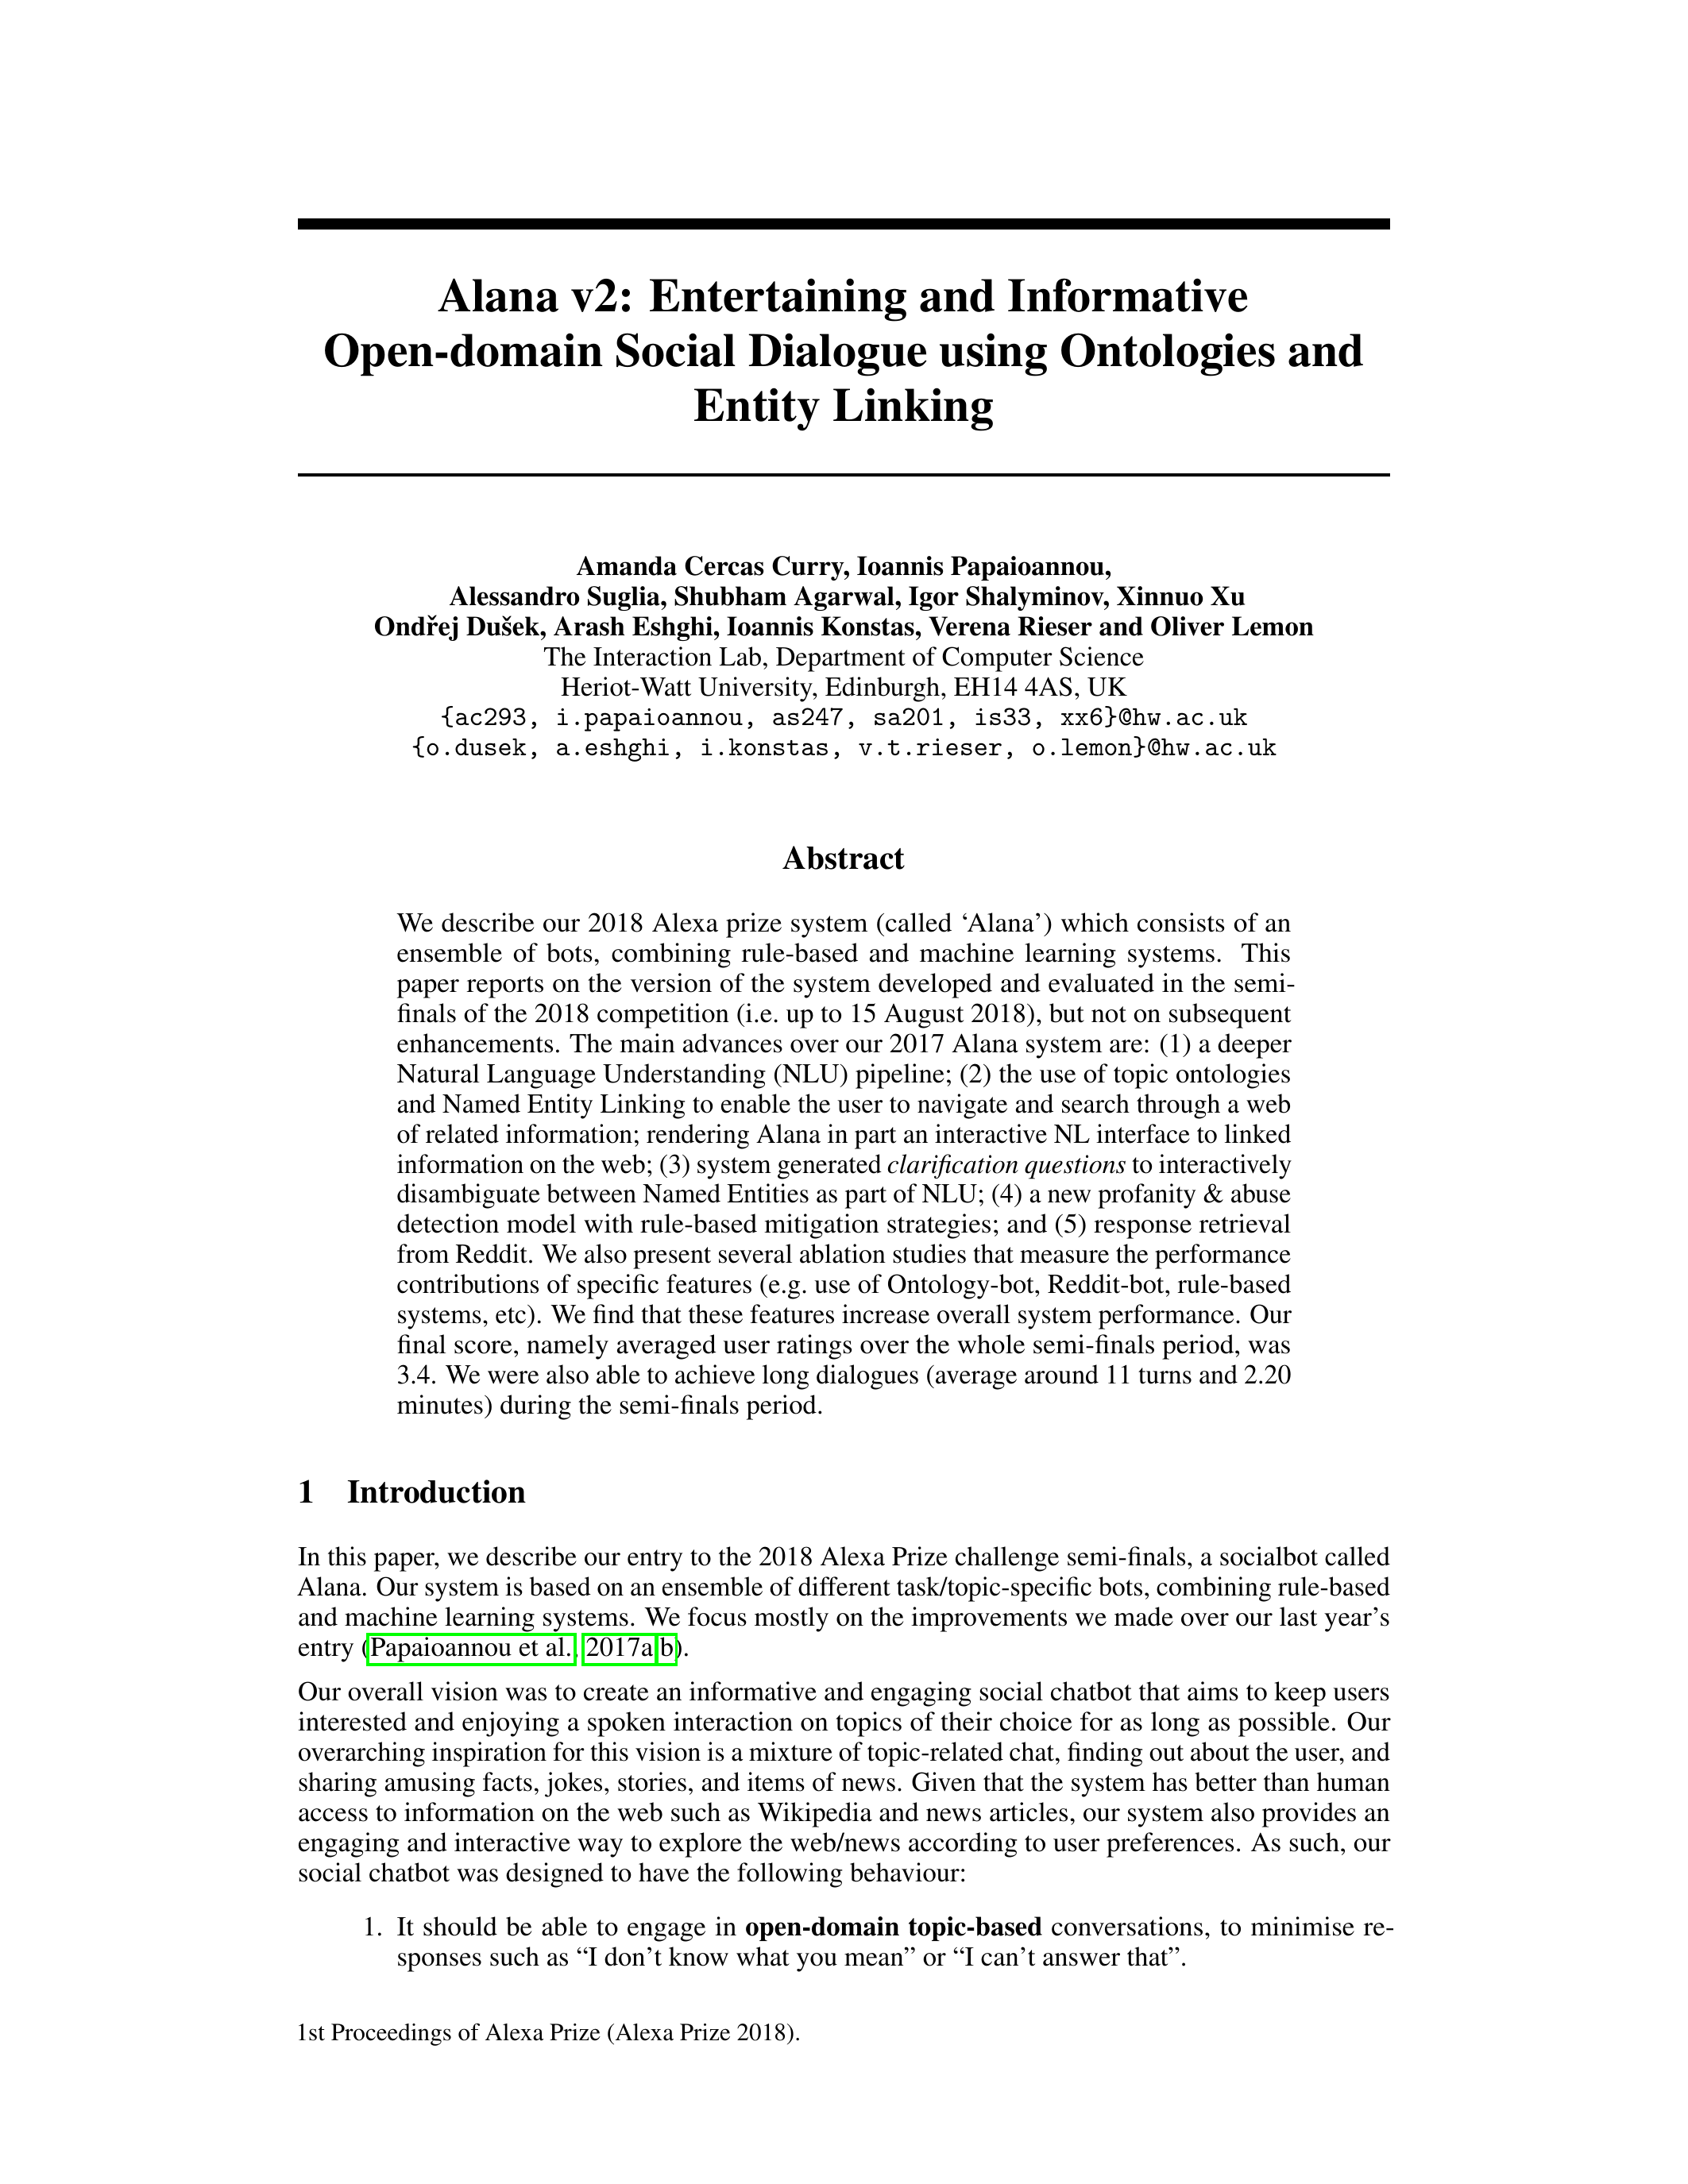}
\includepdf[pages=-,offset=75 -75]{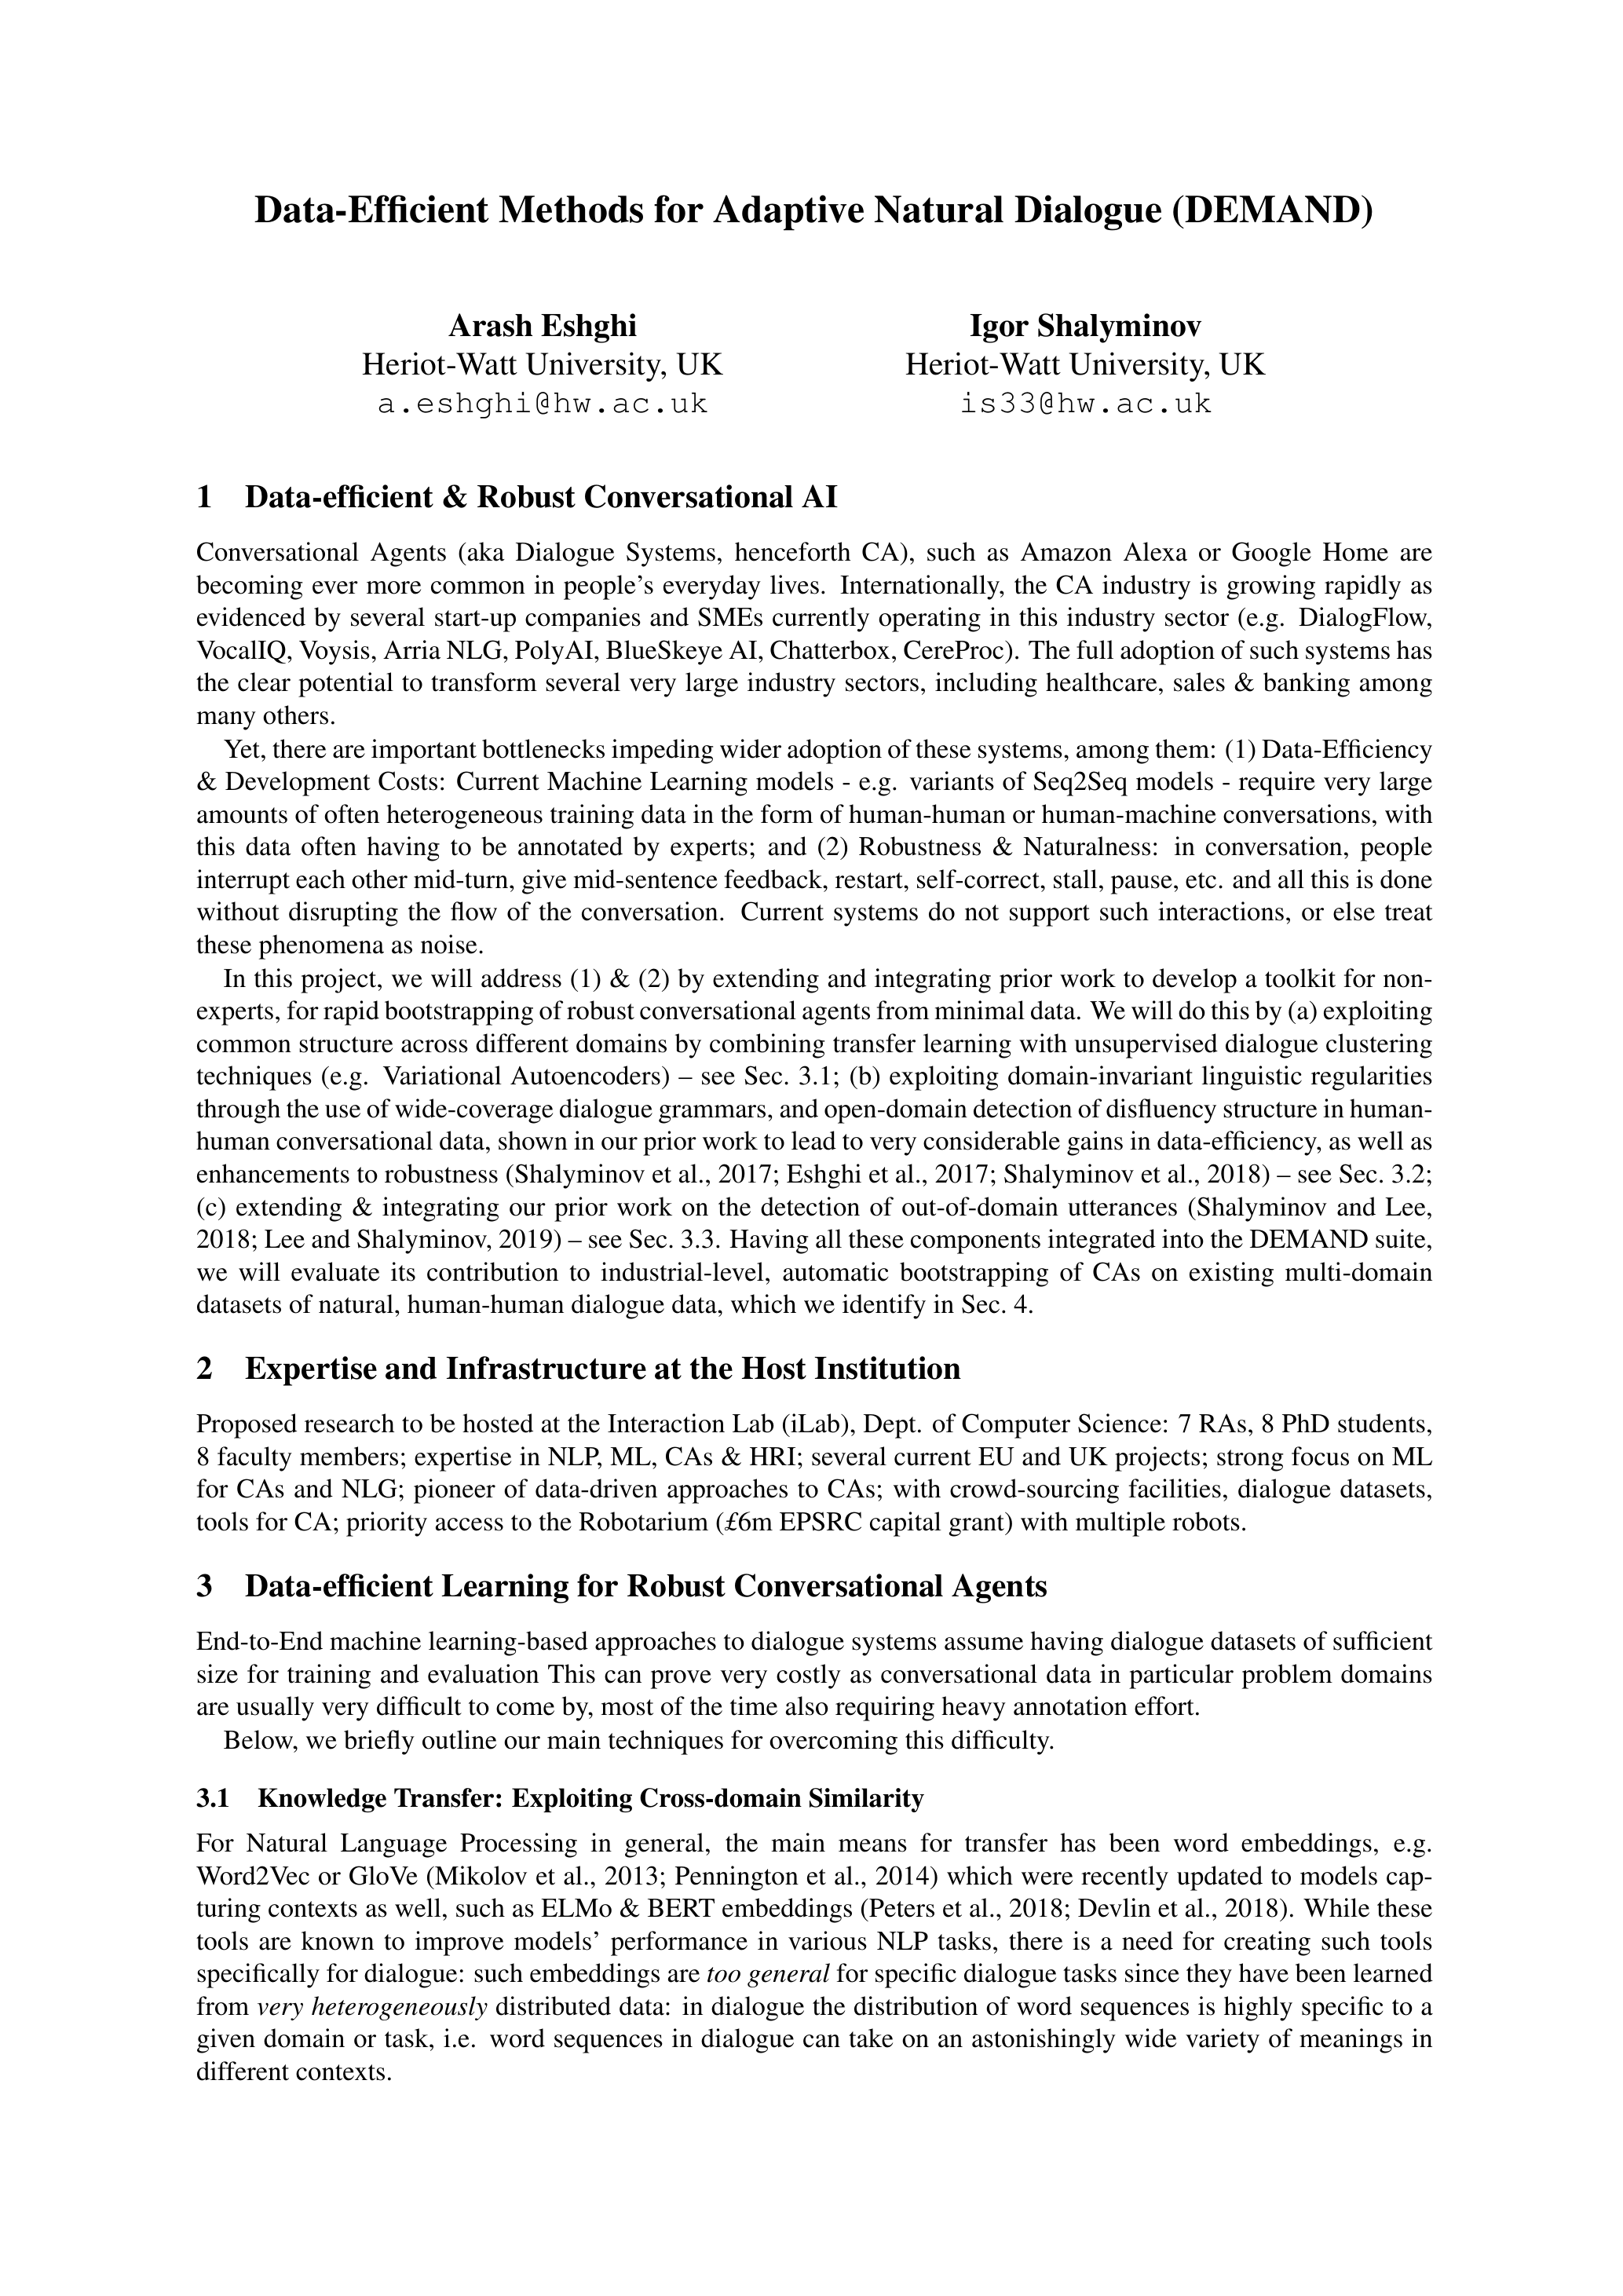}
