# Supplementary material for: Data-Efficient Methods for Dialogue Systems
Source: arXiv:2012.02929 source file (2020-12-05)
Supplement: Supplementary file 3 [file AppendixTemplate.tex]

% Appendix Template

\chapter{Appendix Title Here} % Main appendix title

\label{AppendixX} % Change X to a consecutive letter; for referencing this appendix elsewhere, use \ref{AppendixX}

\lhead{Appendix X. \emph{Appendix Title Here}} % Change X to a consecutive letter; this is for the header on each page - perhaps a shortened title

Write your Appendix content here.
